# Supplementary material for: A Game-Theoretic Approach to the Study of Blockchain's Robustness
Source: arXiv:2411.19175 source file (2024-11-28)
Supplement: Supplementary file 1 [file Pseudo-Randomness.tex]

\chapter{Pseudo-Randomness in Ethereum}\label{chap:Pseudo-Randomness}
